# Supplementary material for: Optimizing Three Critical Factors for Practical and Effective OOD Detection Fine-Tuning
Source: arXiv:2308.01030 source file (2026-09-10)
Supplement: Supplementary file 2 [file 7-supplement.tex]

%%%%%%% supplementary
%%%% energy + ours
% m_in -5 (10) / 
% m_out -23 (10)
% lambda_reg = 0.1 / 0.15(im-balanced)
% lambda_KD = 0.1 / 1 (im-balanced)
% lambda_SC = 1

%%%% balanced energy는 에너지랑 학습 파라미 셋팅 같음.
% gamma = 0.75 형 논문 따름

%%%% oecc + ours
% 15 for c-10 / 30 for c-100 epoch
% balanced
% lambda_reg1 = 0.07
% lambda_reg2 = 0.05

% im-balanced since unstable
% lambda_reg1 = 0.03
% lambda_reg2 = 0.03

% lambda_KD = 1
% lambda_SC = 1

%%%%%%%%%%
% supplementary
% training details
% MOOD benchmark 다른 방법들과 비교 결과
% 4.2절

%%%%%%%%%%%%
% dataset details

% other experiment setting details

% std for comparison with other methods

% visualize 

% logit adjustment + ours
