# Supplementary material for: Optimizing Three Critical Factors for Practical and Effective OOD Detection Fine-Tuning
Source: arXiv:2308.01030 source file (2026-09-10)
Supplement: Supplementary file 8 [file E_comparison_balanced_std.tex]

\begin{table}[h!]
\caption{ Comparison result on MOOD benchmark using CIFAR; Mean and std over 8 random runs are reported; MOOD benchmark detection average (over 11 datasets) performance (AUROC, AP, FPR95) and classification accuracy (ACC) (a): Result on CIFAR10 (b): Result on CIFAR100.}
\begin{subtable}{1.0\linewidth}
\centering
\scriptsize
\caption{}
\label{MOOD_balanced_cifar10_std}
\begin{tabular}{c|c|c|c|c}
\hline

Method         &ACC$\uparrow$     &FPR$\downarrow$     &      AUC$\uparrow$   &     AP$\uparrow$         \\ \hline
MSP~\cite{hendrycks2016baseline}(ST)         & 93.69 $\pm 0.00$         & 30.09 $\pm 0.00$     & 89.53 $\pm 0.00$        & 85.58 $\pm 0.00$         \\
 Energy~\cite{liu2020energy}(ST)      & 93.69 $\pm 0.00$         & 23.64 $\pm 0.00$         & 92.72 $\pm 0.00$       & 90.27 $\pm 0.00$         \\
  OE~\cite{hendrycks2018deep}(scratch)       & 90.12 $\pm 0.69$         & 21.37 $\pm 2.59$         & 93.93 $\pm 0.56$        & 92.99 $\pm 0.66$       \\ 
   EnergyOE~\cite{liu2020energy}(scratch) & 90.50 $\pm 0.35$          & 19.24 $\pm 2.27$     & 94.08 $\pm 0.53$     & 92.91 $\pm 0.71$ \\
   
   WOOD~\cite{katz2022training}(10\%)     & 93.18 $\pm 0.00$    &    16.59 $\pm 0.00$   &   95.43 $\pm 0.00$     &   \textbf{93.98} $\pm 0.00$    \\  
   
   WOOD~\cite{katz2022training}(100\%)     & 93.20 $\pm 0.00$      &    \textbf{16.57} $\pm 0.00$  &   \textbf{95.44} $\pm 0.00$    &   93.94 $\pm 0.00$   \\ 
   
      NTOM~\cite{chen2021atom}(10\%)   & 84.37 $\pm 2.08$         &   46.13 $\pm 3.07$    &   82.37 $\pm 1.56$    &    76.72 $\pm 2.04$   \\
      
      NTOM~\cite{chen2021atom}(100\%)   & \textbf{94.39} $\pm 0.24$  &  23.88 $\pm 0.98$   &   92.23 $\pm 0.38$   &  89.44 $\pm 0.58$ \\\hline   

    OE~\cite{hendrycks2018deep}        & 93.12 $\pm 0.05$ & 18.26 $\pm 0.11$ & 94.79 $\pm 0.03$ & 93.90 $\pm 0.04$          \\ 
    
        \textbf{OE+Ours}           & \textbf{93.38} $\pm 0.10$ & \textbf{14.86} $\pm 0.23$ & \textbf{95.46} $\pm 0.04$ & \textbf{94.53} $\pm 0.09$     \\ \hline
        
        EnergyOE~\cite{liu2020energy}        & 93.33 $\pm 0.09$ & 15.70 $\pm 0.27$ & 95.26 $\pm 0.08$ & 94.50 $\pm 0.12$          \\ 
        \textbf{EnergyOE+Ours}  & \textbf{93.64} $\pm 0.06$ & \textbf{14.40} $\pm 0.45$ & \textbf{95.53} $\pm 0.14$ & \textbf{94.77} $\pm 0.24$      \\ \hline
        
        OECC~\cite{papadopoulos2021outlier}        & 91.81 $\pm 0.24$ & 15.42 $\pm 0.25$ & 94.95 $\pm 0.18$ & 93.27 $\pm 0.69$          \\ 
        
        \textbf{OECC+Ours}    & \textbf{92.18} $\pm 0.28$ & \textbf{14.60} $\pm 0.35$ & \textbf{95.23} $\pm 0.17$ & \textbf{93.66}  $\pm 0.50$   \\ \hline
       \end{tabular}
\end{subtable}
% \begin{subtable}{0.5\linewidth}
\begin{subtable}{1.0\linewidth}
\centering
\scriptsize
%\vspace{0.1cm}
\caption{}
\begin{tabular}{c|c|c|c|c}
\hline

Method         &ACC$\uparrow$     &FPR$\downarrow$     &      AUC$\uparrow$   &     AP$\uparrow$         \\ \hline
MSP~\cite{hendrycks2016baseline}(ST)         & 75.70 $\pm 0.00$         & 59.82 $\pm 0.00$   & 78.12 $\pm 0.00$     & 73.43 $\pm 0.00$         \\
 Energy~\cite{liu2020energy}(ST)      & 75.70 $\pm 0.00$     & 47.23 $\pm 0.00$    & 84.34 $\pm 0.00$  & 79.28 $\pm 0.00$    \\
  OE~\cite{hendrycks2018deep}(scratch)       & 66.47 $\pm 0.45$         & 52.00 $\pm 3.94$    & 84.06 $\pm 1.67$    & 81.18 $\pm 1.88$     \\ 
   EnergyOE~\cite{liu2020energy}(scratch) & 65.92 $\pm 0.77$          & 42.67 $\pm 3.86$   & 86.16 $\pm 1.22$     & 81.84 $\pm 1.53$ \\
   
   WOOD~\cite{katz2022training}(10\%)     & 75.80 $\pm 0.00$    &   \textbf{35.05} $\pm 0.00$    &   \textbf{89.03} $\pm 0.00$     &  \textbf{85.94} $\pm 0.00$   \\  
   
   WOOD~\cite{katz2022training}(100\%)     & \textbf{75.93} $\pm 0.00$   &   35.66 $\pm 0.00$     &   88.82 $\pm 0.00$     &   85.69 $\pm 0.00$    \\ 
   
      NTOM~\cite{chen2021atom}(10\%)   & 49.81 $\pm 4.43$  &  80.57 $\pm 2.92$  & 61.35 $\pm 2.87$     &  56.30 $\pm 2.37$    \\
      
      NTOM~\cite{chen2021atom}(100\%)   &  72.41 $\pm 0.95$    &  52.33 $\pm 1.60$   &   80.98 $\pm 0.79$   & 76.65 $\pm 1.03$   \\\hline  

    OE~\cite{hendrycks2018deep}        & \textbf{73.86} $\pm 0.10$  & 43.42 $\pm 0.20$ & 85.75 $\pm 0.13$ & 81.86 $\pm 0.18$          \\ 
    
        \textbf{OE+Ours}           & 73.13 $\pm 0.19$ & \textbf{36.70} $\pm 0.84$ & \textbf{88.64} $\pm 0.38$ & \textbf{85.38}   $\pm 0.50$       \\ \hline
        
        EnergyOE~\cite{liu2020energy}        & 74.50 $\pm 0.16$ & \textbf{34.96} $\pm 0.89$ & \textbf{89.05} $\pm 0.26$ & 85.46 $\pm 0.38$          \\ 
        \textbf{EnergyOE+Ours}           & \textbf{74.93} $\pm 0.21$ & 35.12 $\pm 1.35$ & \textbf{89.05} $\pm 0.59$ & \textbf{85.47} $\pm 0.92$        \\ \hline
        
        OECC~\cite{papadopoulos2021outlier}        & 69.36 $\pm 0.21$ & 36.98 $\pm 1.39$ & 87.51 $\pm 0.48$ & 82.90 $\pm 0.69$          \\ 
        
        \textbf{OECC+Ours}   & \textbf{72.23} $\pm 0.10$ & \textbf{33.76} $\pm 1.35$ & \textbf{89.51} $\pm 0.40$ & \textbf{86.41}   $\pm 0.61$       \\ \hline
       \end{tabular}
\label{MOOD_balanced_cifar100_std}
\end{subtable}
\label{MOOD_comparison_balanced_std}
\end{table}
