# Supplementary material for: Optimizing Three Critical Factors for Practical and Effective OOD Detection Fine-Tuning
Source: arXiv:2308.01030 source file (2026-09-10)
Supplement: Supplementary file 9 [file E_comparison_imbalanced_std.tex]

\begin{table}[h!]
\caption{Comparison result on MOOD benchmark using LT-CIFAR; Mean and std over 8 random runs are reported; MOOD benchmark detection average (over 11 datasets) performance (AUROC, AP, FPR95) and classification accuracy (ACC) (a): Result on LT-CIFAR10 (b): Result on LT-CIFAR100.}
\begin{subtable}{1.0\linewidth}
\centering
\scriptsize
\caption{}
\label{MOOD_imbalanced_cifar10_std}
\begin{tabular}{c|c|c|c|c}
\hline

Method         &ACC$\uparrow$     &FPR$\downarrow$     &      AUC$\uparrow$   &     AP$\uparrow$         \\ \hline
MSP~\cite{hendrycks2016baseline}(ST)         & 73.28 $\pm 0.00$         & 57.72 $\pm 0.00$   & 75.96 $\pm 0.00$    & 69.93 $\pm 0.00$     \\

 Energy~\cite{liu2020energy}(ST)      & 73.28 $\pm 0.00$ & 43.91 $\pm 0.00$      & 83.88 $\pm 0.00$  & 78.40 $\pm 0.00$     \\
 
  OE~\cite{hendrycks2018deep}(scratch)       & 72.85 $\pm 1.26$        & 35.11 $\pm 2.04$    & 88.07 $\pm 0.77$    & 82.79 $\pm 1.41$      \\ 
  
   EnergyOE~\cite{liu2020energy}(scratch) & 73.40 $\pm 0.52$        & \textbf{33.99} $\pm 1.33$   & 84.45 $\pm 0.86$      & 74.61 $\pm 1.86$ \\
   
   PASCL~\cite{wang2022partial}     & \textbf{77.08} $\pm 1.01$    &  35.88 $\pm 1.26$  & \textbf{88.90} $\pm 0.56$   &  \textbf{ 85.42} $\pm 1.14$     \\   
   
      OS~\cite{wei2022open}   & 77.04 $\pm 0.54$   &   35.21 $\pm 1.94$  & 88.32 $\pm 0.73$       & 82.19 $\pm 1.60$   \\ \hline   

    OE~\cite{hendrycks2018deep}        & 69.73 $\pm 0.12$ & 40.71 $\pm 0.20$ & 87.39 $\pm 0.07$ & 85.48 $\pm 0.08$    \\
    
        \textbf{OE+Ours}           & \textbf{77.66} $\pm 0.11$ & \textbf{30.46} $\pm 0.43$ & \textbf{91.14} $\pm 0.09$ & \textbf{89.88}  $\pm 0.11$        \\ \hline
        
        EnergyOE~\cite{liu2020energy}    & 74.77 $\pm 0.20$ & 31.22 $\pm 0.57$ & 90.99 $\pm 0.14$ & \textbf{89.87} $\pm 0.17$ \\ 
        
        \textbf{EnergyOE+Ours}           & \textbf{78.18} $\pm 0.13$ & \textbf{28.67} $\pm 0.71$ & \textbf{91.29} $\pm 0.19$ & 89.73 $\pm 0.25$         \\ \hline
        
        OECC~\cite{papadopoulos2021outlier}        & 62.01 $\pm 0.26$ & 34.78 $\pm 0.23$ & 89.48 $\pm 0.08$ & \textbf{87.94} $\pm 0.17$  \\ 
        
        \textbf{OECC+Ours}     & \textbf{75.23} $\pm 0.16$ & \textbf{30.06} $\pm 0.89$ & \textbf{90.53} $\pm 0.25$ & 87.73  $\pm 0.51$   \\\hline 
        
        BEnergyOE~\cite{choi2023}   & 76.30 $\pm 0.24$ & 27.59 $\pm 0.59$ & 91.91 $\pm 0.15$ & \textbf{90.46} $\pm 0.18$  \\ 
        
        \textbf{BEnergyOE   +Ours}   & \textbf{78.13} $\pm 0.18$ & \textbf{25.99} $\pm 0.48$ & \textbf{92.09} $\pm 0.13$ & \textbf{90.46} $\pm 0.19$         \\         
        \hline
       \end{tabular}
\end{subtable}
\begin{subtable}{1.0\linewidth}
\centering
\scriptsize
%\vspace{0.1cm}
\caption{}
\begin{tabular}{c|c|c|c|c}
\hline
Method         &ACC$\uparrow$     &FPR$\downarrow$     &      AUC$\uparrow$   &     AP$\uparrow$         \\ \hline
MSP~\cite{hendrycks2016baseline}(ST)         & 40.22 $\pm 0.00$         & 78.68 $\pm 0.00$     & 64.16 $\pm 0.00$       & 58.89 $\pm 0.00$         \\

 Energy~\cite{liu2020energy}(ST)      & 40.22 $\pm 0.00$   & 69.56 $\pm 0.00$  & 69.66 $\pm 0.00$   & 63.17 $\pm 0.00$   \\
 
  OE~\cite{hendrycks2018deep}(scratch)       & 41.31 $\pm 0.66$         & 60.36 $\pm 3.73$    & 76.95 $\pm 2.03$     & 71.28 $\pm 2.46$         \\ 
  
   EnergyOE~\cite{liu2020energy}(scratch) & 40.78 $\pm 0.33$        &  \textbf{52.20} $\pm 2.07$ & \textbf{79.41} $\pm 1.16$   & \textbf{72.96} $\pm 1.59$ \\
   
   PASCL~\cite{wang2022partial}      & \textbf{43.10}  $\pm 0.47$      &    65.32 $\pm 1.03$     &   74.25  $\pm 0.87$     & 68.35 $\pm 1.02$    \\   
   
      OS~\cite{wei2022open}   & 39.96 $\pm 0.60$   & 58.56 $\pm 1.86$   &   77.25 $\pm 1.49$  &      70.72 $\pm 2.06$  \\ \hline   

    OE~\cite{hendrycks2018deep}        & 38.93 $\pm 0.07$ & 66.27 $\pm 0.16$ & 74.36 $\pm 0.11$ & 69.28 $\pm 0.12$          \\
    
        \textbf{OE+Ours}    & \textbf{39.73} $\pm 0.09$ & \textbf{51.04} $\pm 0.51$ & \textbf{81.43} $\pm 0.22$ & \textbf{76.56} $\pm 0.24$    \\ \hline
        
        EnergyOE~\cite{liu2020energy}        & 40.54 $\pm 0.08$ & 50.05 $\pm 0.30$ & 81.82 $\pm 0.18$ & \textbf{77.17} $\pm 0.26$          \\ 
        
        \textbf{EnergyOE+Ours}           & \textbf{40.76} $\pm 0.13$ & \textbf{47.81} $\pm 0.42$ & \textbf{82.31} $\pm 0.23$ & 76.49 $\pm 0.35$         \\ \hline
        
        OECC~\cite{papadopoulos2021outlier}        & 31.08 $\pm 0.11$ & 50.75 $\pm 0.20$ & 81.79 $\pm 0.12$ & \textbf{77.90} $\pm 0.17$  \\ 
        
        \textbf{OECC+Ours}      & \textbf{39.77} $\pm 0.13$ & \textbf{47.28} $\pm 0.40$ & \textbf{82.52} $\pm 0.12$ & 77.68 $\pm 0.18$   \\\hline 
        
        BEnergyOE~\cite{choi2023}   & 40.78 $\pm 0.21$ & 45.37 $\pm 0.42$ & 83.64 $\pm 0.21$ & 79.21 $\pm 0.28$    \\ 
        
        \textbf{BEnergyOE   +Ours}  & \textbf{43.45} $\pm 0.14$ & \textbf{43.06} $\pm 0.44$ & \textbf{84.78} $\pm 0.17$ & \textbf{80.68} $\pm 0.27$         \\         
        \hline
       \end{tabular}
\label{MOOD_imbalanced_cifar100_std}
\end{subtable}
\label{MOOD_comparison_imbalanced_std}
\end{table}
