# Supplementary material for: Optimizing Three Critical Factors for Practical and Effective OOD Detection Fine-Tuning
Source: arXiv:2308.01030 source file (2026-09-10)
Supplement: Supplementary file 10 [file E_comparsion_balanced.tex]

\begin{table}[h!]
\captionsetup{font=footnotesize}
\caption{ Comparison result on MOOD benchmark using CIFAR; Mean over 8 random runs are reported; MOOD benchmark detection average (over 11 datasets) performance (AUROC, AP, FPR95) and classification accuracy (ACC) (a): Result on CIFAR10 (b): Result on CIFAR100.}
\begin{subtable}{0.5\linewidth}
\centering
\scriptsize
\caption{}
\label{MOOD_balanced_cifar10}
\begin{tabular}{c|c|c|c|c}
\hline

Method         &ACC$\uparrow$     &FPR$\downarrow$     &      AUC$\uparrow$   &     AP$\uparrow$         \\ \hline
MSP~\cite{hendrycks2016baseline}(ST)         & 93.69          & 30.09      & 89.53         & 85.58          \\
 Energy~\cite{liu2020energy}(ST)      & 93.69          & 23.64          & 92.72        & 90.27          \\
  OE~\cite{hendrycks2018deep}(scratch)       & 90.12          & 21.37          & 93.09         & 92.99        \\ 
   EnergyOE~\cite{liu2020energy}(scratch) & 90.50          & 19.24     & 94.08      & 92.91 \\
   
   WOOD~\cite{katz2022training}(10\%)     & 93.18    &    16.59    &   95.43      &   \textbf{93.98}     \\  
   
   WOOD~\cite{katz2022training}(100\%)     & 93.20       &    \textbf{16.57}   &   \textbf{95.44}     &   93.94    \\ 
   
      NTOM~\cite{chen2021atom}(10\%)   & 84.37          &   46.13     &   82.37     &    76.72    \\
      
      NTOM~\cite{chen2021atom}(100\%)   & \textbf{94.39}   &  23.88    &   92.23    &  89.44  \\\hline   

    OE~\cite{hendrycks2018deep}        & 93.12 & 18.26 & 94.79 & 93.90          \\ 
        \textbf{OE+Ours}           & \textbf{93.38} & \textbf{14.86} & \textbf{95.46} & \textbf{94.53}      \\ \hline
        
        EnergyOE~\cite{liu2020energy}        & 93.33 & 15.70 & 95.26 & 94.50          \\ 
        \textbf{EnergyOE+Ours}  & \textbf{93.64} & \textbf{14.40} & \textbf{95.53} & \textbf{94.77}       \\ \hline
        
        OECC~\cite{papadopoulos2021outlier}        & 91.81 & 15.42 & 94.95 & 93.27          \\ 
        \textbf{OECC+Ours}    & \textbf{92.18} & \textbf{14.60} & \textbf{95.23} & \textbf{93.66}     \\ \hline
       \end{tabular}
\end{subtable}
\begin{subtable}{0.5\linewidth}
\centering
\scriptsize
%\vspace{0.1cm}
\caption{}
\begin{tabular}{c|c|c|c|c}
\hline

Method         &ACC$\uparrow$     &FPR$\downarrow$     &      AUC$\uparrow$   &     AP$\uparrow$         \\ \hline
MSP~\cite{hendrycks2016baseline}(ST)         & 75.70          & 59.82    & 78.12      & 73.43          \\
 Energy~\cite{liu2020energy}(ST)      & 75.70      & 47.23     & 84.34   & 79.28     \\
  OE~\cite{hendrycks2018deep}(scratch)       & 66.47          & 52.00     & 84.06     & 81.18      \\ 
   EnergyOE~\cite{liu2020energy}(scratch) & 65.92          & 42.67    & 86.16      & 81.84 \\
   
   WOOD~\cite{katz2022training}(10\%)     & 75.80     &   \textbf{35.05}     &   \textbf{89.03}      &  \textbf{85.94}    \\  
   
   WOOD~\cite{katz2022training}(100\%)     & \textbf{75.93}    &   35.66      &   88.82      &   85.69     \\ 
   
      NTOM~\cite{chen2021atom}(10\%)   & 49.81  &  80.57   & 61.35     &      56.30    \\
      
      NTOM~\cite{chen2021atom}(100\%)   &  72.41    &  52.33    &   80.98    & 76.65   \\\hline  

    OE~\cite{hendrycks2018deep}        & \textbf{73.86}  & 43.42 & 85.75 & 81.86          \\ 
    
        \textbf{OE+Ours}           & 73.13 & \textbf{36.70} & \textbf{88.64} & \textbf{85.38}          \\ \hline
        
        EnergyOE~\cite{liu2020energy}        & 74.50 & \textbf{34.96} & \textbf{89.05} & 85.46          \\ 
        \textbf{EnergyOE+Ours}           & \textbf{74.93} & 35.12 & \textbf{89.05} & \textbf{85.47}         \\ \hline
        
        OECC~\cite{papadopoulos2021outlier}        & 69.36 & 36.98 & 87.51 & 82.90          \\ 
        \textbf{OECC+Ours}   & \textbf{72.23} & \textbf{33.76} & \textbf{89.51} & \textbf{86.41}          \\ \hline
       \end{tabular}
\label{MOOD_balanced_cifar100}
\end{subtable}
\label{MOOD_comparison_balanced}
\end{table}
