# Supplementary material for: Optimizing Three Critical Factors for Practical and Effective OOD Detection Fine-Tuning
Source: arXiv:2308.01030 source file (2026-09-10)
Supplement: Supplementary file 11 [file E_comparsion_imbalanced.tex]

\begin{table}[h!]
\captionsetup{font=footnotesize}
\caption{Comparison result on MOOD benchmark using LT-CIFAR; Mean over 8 random runs are reported; MOOD benchmark detection average (over 11 datasets) performance (AUROC, AP, FPR95) and classification accuracy (ACC) (a): Result on LT-CIFAR10 (b): Result on LT-CIFAR100.}
\begin{subtable}{0.5\linewidth}
\centering
\scriptsize
\caption{}
\label{MOOD_imbalanced_cifar10}
\begin{tabular}{c|c|c|c|c}
\hline

Method         &ACC$\uparrow$     &FPR$\downarrow$     &      AUC$\uparrow$   &     AP$\uparrow$         \\ \hline
MSP~\cite{hendrycks2016baseline}(ST)         & 73.28          & 57.72    & 75.96     & 69.93      \\

 Energy~\cite{liu2020energy}(ST)      & 73.28 & 43.91       & 83.88   & 78.40      \\
 
  OE~\cite{hendrycks2018deep}(scratch)       & 72.85         & 35.11     & 88.07     & 82.79       \\ 
  
   EnergyOE~\cite{liu2020energy}(scratch) & 73.40         & \textbf{33.99}   & 84.45       & 74.61 \\
   
   PASCL~\cite{wang2022partial}     & \textbf{77.08}     &  35.88   & \textbf{88.90}    &  \textbf{ 85.42}     \\   
   
      OS~\cite{wei2022open}   & 77.04    &   35.21  & 88.32        & 82.19    \\ \hline   

    OE~\cite{hendrycks2018deep}        & 69.73 & 40.71 & 87.39 & 85.48    \\
    
        \textbf{OE+Ours}           & \textbf{77.66} & \textbf{30.46} & \textbf{91.14} & \textbf{89.88}          \\ \hline
        
        EnergyOE~\cite{liu2020energy}    & 74.77 & 31.22 & 90.99 & \textbf{89.87} \\ 
        
        \textbf{EnergyOE+Ours}           & \textbf{78.18} & \textbf{28.67} & \textbf{91.29} & 89.73          \\ \hline
        
        OECC~\cite{papadopoulos2021outlier}        & 62.01 & 34.78 & 89.48 & \textbf{87.94}   \\ 
        
        \textbf{OECC+Ours}     & \textbf{75.23} & \textbf{30.06} & \textbf{90.53} & 87.73     \\\hline 
        
        BEnergyOE~\cite{choi2023}   & 76.30 & 27.59 & 91.91 & \textbf{90.46}  \\ 
        
        \textbf{BEnergyOE   +Ours}   & \textbf{78.13} & \textbf{25.99} & \textbf{92.09} & \textbf{90.46}          \\         
        \hline
       \end{tabular}
\end{subtable}
\begin{subtable}{0.5\linewidth}
\centering
\scriptsize
%\vspace{0.1cm}
\caption{}
\begin{tabular}{c|c|c|c|c}
\hline
Method         &ACC$\uparrow$     &FPR$\downarrow$     &      AUC$\uparrow$   &     AP$\uparrow$         \\ \hline
MSP~\cite{hendrycks2016baseline}(ST)         & 40.22          & 76.68      & 64.16        & 58.89          \\

 Energy~\cite{liu2020energy}(ST)      & 40.22    & 69.56   & 69.66   & 63.17    \\
 
  OE~\cite{hendrycks2018deep}(scratch)       & 41.31          & 60.36     & 76.95      & 71.28          \\ 
  
   EnergyOE~\cite{liu2020energy}(scratch) & 40.78         &  \textbf{52.20}  & \textbf{79.41}    & \textbf{72.96} \\
   
   PASCL~\cite{wang2022partial}      & \textbf{43.10}          &    65.32      &   74.25       & 68.35     \\   
   
      OS~\cite{wei2022open}   & 39.96    & 58.56    &   77.25   &      70.72   \\ \hline   

    OE~\cite{hendrycks2018deep}        & 38.93 & 66.27 & 74.36 & 69.28          \\
    
        \textbf{OE+Ours}    & \textbf{39.7}3 & \textbf{51.04} & \textbf{81.43} & \textbf{76.56}     \\ \hline
        
        EnergyOE~\cite{liu2020energy}        & 40.54 & 50.05 & 81.82 & \textbf{77.17}          \\ 
        
        \textbf{EnergyOE+Ours}           & \textbf{40.76} & \textbf{47.81} & \textbf{82.31} & 76.49          \\ \hline
        
        OECC~\cite{papadopoulos2021outlier}        & 31.08 & 50.75 & 81.79 & \textbf{77.90}   \\ 
        
        \textbf{OECC+Ours}      & \textbf{39.77} & \textbf{47.28} & \textbf{82.52} & 77.68    \\\hline 
        
        BEnergyOE~\cite{choi2023}   & 40.78 & 45.37 & 83.64 & 79.21    \\ 
        
        \textbf{BEnergyOE   +Ours}  & \textbf{43.45} & \textbf{43.06} & \textbf{84.78} & \textbf{80.68}          \\         
        \hline
       \end{tabular}
\label{MOOD_imbalanced_cifar100}
\end{subtable}
\label{MOOD_comparison_imbalanced}
\end{table}
