# Supplementary material for: Optimizing Three Critical Factors for Practical and Effective OOD Detection Fine-Tuning
Source: arXiv:2308.01030 source file (2026-09-10)
Supplement: Supplementary file 12 [file D_table.tex]

\begin{table}[h!]
% \captionsetup{font=footnotesize}
\caption{Synthetic benchmark D result test.}
\centering
\scriptsize
\label{syn_D_result}

\begin{tabular}{c|cc|cc|cc}
% \hline
\cline{2-7}
              & \multicolumn{2}{c|}{ACC $\uparrow$}       & \multicolumn{2}{c|}{FPR95 $\downarrow$}     & \multicolumn{2}{c}{AUROC $\uparrow$}     %& \multicolumn{2}{c}{AUPR $\uparrow$}   
              \\ \hline
$D_{in}$         & \multicolumn{1}{c}{OE} & Ours & \multicolumn{1}{c}{OE} & Ours & \multicolumn{1}{c}{OE} & Ours %& \multicolumn{1}{c}{OE} & Ours 
\\ \hline

CIFAR-10      & \multicolumn{1}{c}{93.12 $\pm 0.05$}   & \textbf{93.38} $\pm 0.11$   & \multicolumn{1}{c}{3.97 $\pm 0.14$}   & \textbf{2.18} $\pm 0.31$    & \multicolumn{1}{c}{98.77 $\pm 0.05$}   & \textbf{98.80} $\pm 0.20$   %  & \multicolumn{1}{c}{97.63 $\pm 0.14$}   & 96.24 $\pm 0.58$   
\\ \hline

CIFAR-100     & \multicolumn{1}{c}{\textbf{73.86} $\pm 0.11$}   &  73.13 $\pm 0.20$  & \multicolumn{1}{c}{13.03 $\pm 0.71$}   & \textbf{3.78} $\pm 0.53$  & \multicolumn{1}{c}{91.94 $\pm 0.56$}   & \textbf{98.55} $\pm 0.21$  % & \multicolumn{1}{c}{86.48 $\pm 0.57$}   &  96.48$\pm 0.46
\\ \hline

CIFAR-10(LT)  & \multicolumn{1}{c}{69.73 $\pm 0.13$}   &   \textbf{77.67} $\pm 0.12$   & \multicolumn{1}{c}{30.27 $\pm 0.11$}   & \textbf{20.90} $\pm 0.42$   & \multicolumn{1}{c}{80.03 $\pm 0.36$}   & \textbf{92.32} $\pm 0.29$  % & \multicolumn{1}{c}{77.69 $\pm 0.12$}   &  87.79 $\pm 0.53$  
\\ \hline

CIFAR-100(LT) & \multicolumn{1}{c}{38.93 $\pm 0.08$}   &  \textbf{39.73} $\pm 0.10$   & \multicolumn{1}{c}{72.83 $\pm 1.09$}   & \textbf{28.87} $\pm 2.17$   & \multicolumn{1}{c}{58.62 $\pm 1.31$}   & \textbf{86.40} $\pm 1.48$   %& \multicolumn{1}{c}{52.99 $\pm 0.71$}   &  77.65 $\pm 1.69$   
\\ \hline
\end{tabular}%

\end{table}
