# Supplementary material for: Optimizing Three Critical Factors for Practical and Effective OOD Detection Fine-Tuning
Source: arXiv:2308.01030 source file (2026-09-10)
Supplement: Supplementary file 14 [file E_comparison_imbalanced.tex]

\begin{table}[h!]
\captionsetup{font=footnotesize}
\caption{Comparison result on SYN benchmark using LT-CIFAR; Mean over eight random runs are reported; SYN benchmark detection average (over 3 datasets) performance (AUROC, AP, FPR95) and classification accuracy (ACC) (a): Result on LT-CIFAR10 (b): Result on LT-CIFAR100.}
\begin{subtable}{0.5\linewidth}
\centering
\scriptsize
\caption{}
\label{syn_imbalanced_cifar10}
\begin{tabular}{c|c|c|c|c}
\hline

Method         &ACC$\uparrow$     &FPR$\downarrow$     &      AUC$\uparrow$   &     AP$\uparrow$         \\ \hline
MSP~\cite{hendrycks2016baseline}(ST)         & 73.28          & 48.73   & 76.76   & 70.40     \\

 Energy~\cite{liu2020energy}(ST)      & 73.28 & 45.86    & 74.76  & 63.16   \\
 
  OE~\cite{hendrycks2018deep}(scratch)       & 72.85         & 18.67   & 91.58  & 83.77     \\ 
  
   EnergyOE~\cite{liu2020energy}(scratch) & 73.40         & 13.60   & 93.90    & 88.83 \\
   
   PASCL~\cite{wang2022partial}     & \textbf{77.08}    &  8.49   & \textbf{96.53}  &      \textbf{93.33}    \\   
   
      OS~\cite{wei2022open}   & 77.04   &  \textbf{8.28}  & 94.54  & 86.43   \\ \hline   

    OE~\cite{hendrycks2018deep}        & 69.73 & 30.27 & 80.03 & 77.69    \\
    
        \textbf{OE+Ours}           & \textbf{77.66} & \textbf{20.90} & \textbf{92.32} & \textbf{87.79}     \\ \hline
        
        EnergyOE~\cite{liu2020energy}    & 74.77 & 9.67 & 96.60 & 94.26 \\ 
        
        \textbf{EnergyOE+Ours}    & \textbf{78.18} &\textbf{ 7.79 }& \textbf{97.35} &\textbf{ 95.01}     \\ \hline
        
        OECC~\cite{papadopoulos2021outlier}         & 62.01 & 21.69 & 90.80 & 87.84   \\ 
        
        \textbf{OECC+Ours}     & \textbf{75.23} & \textbf{15.49} & \textbf{94.96} & \textbf{91.70}     \\\hline 
        
        BEnergyOE~\cite{choi2023}  & 76.30 & 7.52 & 97.51 & 95.23  \\ 
        
        \textbf{BEnergyOE   +Ours}   & \textbf{78.13} & \textbf{6.85} & \textbf{97.81} & \textbf{95.58}          \\         
        \hline
       \end{tabular}
\end{subtable}
\begin{subtable}{0.5\linewidth}
\centering
\scriptsize
%\vspace{0.1cm}
\caption{}
\begin{tabular}{c|c|c|c|c}
\hline
Method         &ACC$\uparrow$     &FPR$\downarrow$     &      AUC$\uparrow$   &     AP$\uparrow$         \\ \hline
MSP~\cite{hendrycks2016baseline}(ST)         & 40.22          & 81.44    & 39.46    & 45.89     \\

 Energy~\cite{liu2020energy}(ST)      & 40.22    & 74.98 & 40.91   & 45.33   \\
 
  OE~\cite{hendrycks2018deep}(scratch)       & 41.31          & 22.66    & 85.76    & 72.73        \\ 
  
   EnergyOE~\cite{liu2020energy}(scratch) & 40.78         &  18.54  & 90.10   & 86.07 \\
   
   PASCL~\cite{wang2022partial}     & \textbf{43.10}  & 30.07  & 82.13  & 69.88   \\   
   
      OS~\cite{wei2022open}   & 39.96    & \textbf{16.12}   & \textbf{93.54}   &     \textbf{88.07}   \\ \hline   

    OE~\cite{hendrycks2018deep}        & 38.93 & 72.83 & 58.62 & 52.99    \\
    
        \textbf{OE+Ours}   & \textbf{39.73} & \textbf{28.87} & \textbf{86.40} & \textbf{77.65}    \\ \hline
        
        EnergyOE~\cite{liu2020energy}  & 40.54 & 34.89 & 84.98 & 76.71   \\ 
        
        \textbf{EnergyOE+Ours}    & \textbf{40.76} & \textbf{10.14} & \textbf{97.11} & \textbf{95.81}   \\ \hline
        
        OECC~\cite{papadopoulos2021outlier}        & 31.08 & \textbf{5.91} &\textbf{ 96.87} & \textbf{91.74 }  \\ 
        
        \textbf{OECC+Ours}     & \textbf{39.77}& 10.81 & 94.56 & 88.36    \\\hline 
        
        BEnergyOE~\cite{choi2023}   & 40.78 & 15.84 & 93.82 & 88.40    \\ 
        
        \textbf{BEnergyOE   +Ours}  & \textbf{43.45} & \textbf{3.68} & \textbf{98.21} &\textbf{ 94.90 }         \\         
        \hline
       \end{tabular}
\label{balanced_cifar100}
\end{subtable}
\end{table}
