# Supplementary material for: Optimizing Three Critical Factors for Practical and Effective OOD Detection Fine-Tuning
Source: arXiv:2308.01030 source file (2026-09-10)
Supplement: Supplementary file 16 [file E_comparsion_balanced.tex]

\begin{table}[h!]
\captionsetup{font=footnotesize}
\caption{Comparison result on SYN benchmark using CIFAR; Mean over eight random runs are reported; SYN benchmark detection average (over 3 datasets) performance (AUROC, AP, FPR95) and classification accuracy (ACC) (a): Result on CIFAR10 (b): Result on CIFAR100.}
\begin{subtable}{0.5\linewidth}
\centering
\scriptsize
\caption{}
\label{syn_balanced_cifar10}
\begin{tabular}{c|c|c|c|c}
\hline

Method         &ACC$\uparrow$     &FPR$\downarrow$     &      AUC$\uparrow$   &     AP$\uparrow$         \\ \hline
MSP~\cite{hendrycks2016baseline}(ST)         & 93.69          & 20.07      & 90.73      & 83.14       \\

 Energy~\cite{liu2020energy}(ST)      & 93.69          & 14.36   & 93.38   & 86.37     \\
 
  OE~\cite{hendrycks2018deep}(scratch)       & 90.12          & 2.39     & \textbf{99.40}     & \textbf{99.14}       \\ 
  
   EnergyOE~\cite{liu2020energy}(scratch) & 90.50          & \textbf{1.82}   & 99.26  & 98.44 \\
   
   WOOD~\cite{katz2022training}(10\%)     & 93.18    &  4.05   &  98.69  &   97.20  \\  
   
   WOOD~\cite{katz2022training}(100\%)     & 93.2   &  3.80  & 98.72  &   97.16   \\ 
   
      NTOM~\cite{chen2021atom}(10\%)   & 84.37   &  27.65   &  87.18     & 80.12    \\
      
      NTOM~\cite{chen2021atom}(100\%)   & \textbf{94.39}   & 10.33 & 95.14  &  90.80  \\\hline   

    OE~\cite{hendrycks2018deep}   & 93.12 & 3.97 & 98.77 & \textbf{97.63}   \\ 
    
        \textbf{OE+Ours}     & \textbf{93.38} & \textbf{2.18} &\textbf{98.80} & 96.24  \\ \hline
        
        EnergyOE~\cite{liu2020energy}        & 93.33 & 1.67 &\textbf{ 99.28 }& \textbf{97.90}     \\ 
        
        \textbf{EnergyOE+Ours}           & \textbf{93.64} & \textbf{1.52} & 99.24 & 97.63          \\ \hline
        
        OECC~\cite{papadopoulos2021outlier}     & 91.81 & \textbf{1.49} & \textbf{99.31} & \textbf{97.87}    \\ 
        
        \textbf{OECC+Ours}    & \textbf{92.18} & 3.86 & 97.55 & 93.11  \\ \hline
       \end{tabular}
\end{subtable}
\begin{subtable}{0.5\linewidth}
\centering
\scriptsize
%\vspace{0.1cm}
\caption{}
\begin{tabular}{c|c|c|c|c}
\hline

Method         &ACC$\uparrow$     &FPR$\downarrow$     &      AUC$\uparrow$   &     AP$\uparrow$         \\ \hline
MSP~\cite{hendrycks2016baseline}(ST)         & 75.70          & 39.91    & 78.27   & 67.49   \\

 Energy~\cite{liu2020energy}(ST)      & 75.70  & 49.52   & 61.58   & 56.77  \\
 
  OE~\cite{hendrycks2018deep}(scratch)       & 66.47   & 13.67  & 93.96  & \textbf{93.09}      \\ 
  
   EnergyOE~\cite{liu2020energy}(scratch) & 65.92          & \textbf{10.99}    & \textbf{95.24}     & 92.93 \\
   
   WOOD~\cite{katz2022training}(10\%)     & 75.8     &  35.13 & 73.93   &  69.35 \\  
   
   WOOD~\cite{katz2022training}(100\%)     & \textbf{75.93}    &   35.16  &   73.96      & 69.41    \\ 
   
      NTOM~\cite{chen2021atom}(10\%)   & 49.81  & 74.72  & 43.00    &      49.42  \\
      
      NTOM~\cite{chen2021atom}(100\%)   &  72.41  & 37.15  & 80.21    & 72.86  \\\hline  

    OE~\cite{hendrycks2018deep}   & \textbf{73.86}  & 13.03 & 91.94 & 86.48     \\ 
    
        \textbf{OE+Ours}    & 73.13 & \textbf{3.78} & \textbf{98.55} & \textbf{96.48}    \\ \hline
        
        EnergyOE~\cite{liu2020energy}   & 74.50 & 5.34 & 98.02 & 95.82  \\
        
        \textbf{EnergyOE+Ours}           & \textbf{74.93} & \textbf{2.85} & \textbf{99.17} & \textbf{98.37}        \\ \hline
        
        OECC~\cite{papadopoulos2021outlier}        & 69.36 & 6.71 & 96.67 & 92.23          \\ 
        \textbf{OECC+Ours}     & \textbf{72.23} & \textbf{5.94} & \textbf{96.98} & \textbf{93.08}     \\ \hline
       \end{tabular}
\label{balanced_cifar100}
\end{subtable}
\end{table}
